# Supplementary material for: Cross-lingual Transfer Can Worsen Bias in Sentiment Analysis
Source: arXiv:2305.12709 source file (2023-05-22)
Supplement: Supplementary file 1 [file all_confusion_appendix_short.tex]

\begin{figure*}[ht]
    \centering
    \begin{subfigure}[b]{\textwidth}
        \includegraphics[height=4cm]{figures/all_confusion_short/ja_all_confusion_short.pdf}
        \caption{Japanese (ja)}
        \label{fig:b}
    \end{subfigure}
    ~
    \begin{subfigure}[b]{\textwidth}
        \includegraphics[height=4cm]{figures/all_confusion_short/de_all_confusion_short.pdf}
        \caption{German (de)}
        \label{fig:}
    \end{subfigure}
    ~ 
    \begin{subfigure}[b]{\textwidth}
        \includegraphics[height=4cm]{figures/all_confusion_short/es_all_confusion_short.pdf}
        \caption{Spanish (es)}
        \label{fig:}
    \end{subfigure}
    ~ 
    \begin{subfigure}[b]{\textwidth}
        \includegraphics[height=4cm]{figures/all_confusion_short/en_all_confusion_short.pdf}
        \caption{English (en)}
        \label{fig:}
    \end{subfigure}
    ~
    \begin{subfigure}[b]{\textwidth}
        \includegraphics[height=2cm]{figures/all_confusion_short/zh_all_confusion_short.pdf}
        \caption{Chinese (zh\_cn)}
        \label{fig:}
    \end{subfigure}
    \caption{All confusion matrices for experiments in this paper. Higher colour saturation in the lower triangle is bias against the minoritised group, in the upper triangle is bias against the privileged group. Saturations are not normalised across all languages and models; this is not a proxy for aggregate comparative bias, it shows the pattern across sentiment scores.} 
    \label{fig:all_confusion_short}
\end{figure*}
